# Supplementary material for: One Polyp Identifies All: One-Shot Polyp Segmentation with SAM via Cascaded Priors and Iterative Prompt Evolution
Source: arXiv:2507.16337 source file (2025-07-22)
Supplement: Supplementary file 1 [file X_suppl.tex]

\clearpage
\setcounter{page}{1}
\setcounter{page}{1}
\setcounter{section}{0}
\setcounter{figure}{0}
\setcounter{table}{0}
\maketitlesupplementary

% \section{More Implementation Details}
% \label{sec:imple_detail}
% In lesion scaling, we 
\section{Extended Experimental Results}
Due to page limitations, only experimental results from the first three centers from PolypGen were presented in the main text. The experimental results from Centers 4 and 5 are included in the supplementary materials \cref{tab:con_comparison}. The results demonstrate that OP-SAM consistently outperforms state-of-the-art (SOTA) methods across these two additional centers. Notably, in Center 4, the proposed method achieved an 11.89 improvement in IoU compared to SOTA methods. Furthermore, the proposed method exhibits superior robustness, achieving optimal performance across both centers.
\label{sec:more_exp}
\begin{table}[h]
\centering
\begin{tabular}{l|c c|c c}
\hline
\multirow{3}{*}{Method} & \multicolumn{4}{c}{PolypGen} \\
\cline{2-5}
 & \multicolumn{2}{c|}{Center 4} & \multicolumn{2}{c}{Center 5} \\
\cline{2-5}
 & IoU & Dice & IoU & Dice\\
\hline
% PerSAM\cite{zhang2023personalize} & 10.16 & 15.06 & 14.01 & 22.48 \\
% \hspace{1em}\textit{+ EPE} & - & - & - & - & - & - & - & - & - & - & - & - \\
PerSAM & 23.30 & 27.30 & 42.26 & 49.45 \\
PerSAM-f & 24.36 & 27.94 & 26.75 & 32.99 \\
Matcher & 26.31 & 33.94 & 38.78 & 47.71 \\
ProtoSAM & 27.16 & 36.28 & 30.91 & 41.19 \\
% \hspace{1em}\textit{+ EPE} & - & - & - & - & - & - & - & - & - & - & - & - \\
\hline
OP-SAM(ours)& \textbf{39.05} & \textbf{44.76} & \textbf{48.63} & \textbf{56.77} \\
\hline
\end{tabular}
\caption{Continued quantitative performance comparison of the proposed method against state-of-the-art methods on PolypGen Dataset.}
\label{tab:con_comparison}
\end{table}
\section{Feature Selection Ablations}
Throughout all experiments presented in the main text, value embeddings from the final attention module of the DINOv2 model were extracted for cross-correlation computation. Here, we investigate the impact of different feature embeddings on the final segmentation results, see \cref{tab:feats_aba}. The query, key, and value embeddings from the final attention module, as well as the feature embeddings output, are extracted and evaluated separately. The experimental results indicate that utilizing value embeddings for cross-correlation yields the highest accuracy. This finding aligns with previous literature suggesting that value embeddings most effectively capture the semantic features of each patch.
\begin{table}[h]
\centering
\begin{tabular}{c | c c c c | c c }
\hline
 \multirow{2}{*}{Method} & \multicolumn{4}{c|}{Modules} & \multirow{2}{*}{IoU} & \multirow{2}{*}{Dice} \\
\cline{2-5}
 & Q & K & V & Feats &  & \\
\hline
\multirow{4}{*}{OP-SAM} & \ding{52} & & & & 70.61 & 79.16\\
& & \ding{52}& & & 68.47 & 77.27 \\
& & & \ding{52} & & \textbf{76.93} & \textbf{84.53}  \\
& & & & \ding{52} & 74.00 & 82.15  \\
\hline
\end{tabular}
\caption{Ablation studies of feature selections, Q, K, V, Feats denote query, key, value features and the final features output from the image encoder.}
\label{tab:feats_aba}
\end{table}
\section{Self-refinement Ablations}
Additional ablation experiments are conducted to investigate the impact of self-correlation in prior refinement. In the main text, the number of self-refinement iterations ($\rho$) was set to 2. The effect of varying iteration numbers from 1 to 4 on the final segmentation results is subsequently evaluated \cref{tab:self_corr_aba}. The experimental results demonstrate that segmentation accuracy initially increases and then decreases as the number of self-refinement iterations increases, reaching peak performance at 2 iterations. This phenomenon can be attributed to the fact that increasing the number of self-refinement iterations inevitably introduces erroneous relationships from self-correlation.
\begin{table}[h]
\centering
\begin{tabular}{c | c | c c }
\hline
Method & Iter\_num & IoU & Dice \\
\hline
\multirow{4}{*}{OP-SAM} & 1 & 75.08 & 82.86\\
& 2 & \textbf{76.93} & \textbf{84.53} \\
& 3 & 71.89 & 80.14  \\
& 4 & 54.96 & 65.71  \\
\hline
\end{tabular}
\caption{Ablation studies of self-refinement iterations.}
\label{tab:self_corr_aba}
\end{table}
\section{Inference Time Comparison}
Finally, a comparative analysis of inference time is conducted between OP-SAM and SOTA methods \cref{tab:time}. The results indicate that OP-SAM achieves the fastest inference speed among all methods except PerSAM, while PerSAM exhibits significantly lower inference accuracy than other methods. By constraining the iteration number in the prompting module, OP-SAM achieves a superior balance between accuracy and inference speed.
\begin{table}[h]
\centering
\begin{tabular}{c | c c c c }
\hline
Method & PerSAM & Matcher & ProtoSAM & Ours \\
\hline
Time/s & 0.236 & 0.717 & 0.866 & 0.466\\
\hline
\end{tabular}
\caption{Inference time comparison.}
\label{tab:time}
\end{table}

\section{More Visual Results}
\label{sec:more_vis}
\begin{figure*}[h]
  \centering
   \includegraphics[width=0.9\textwidth]{{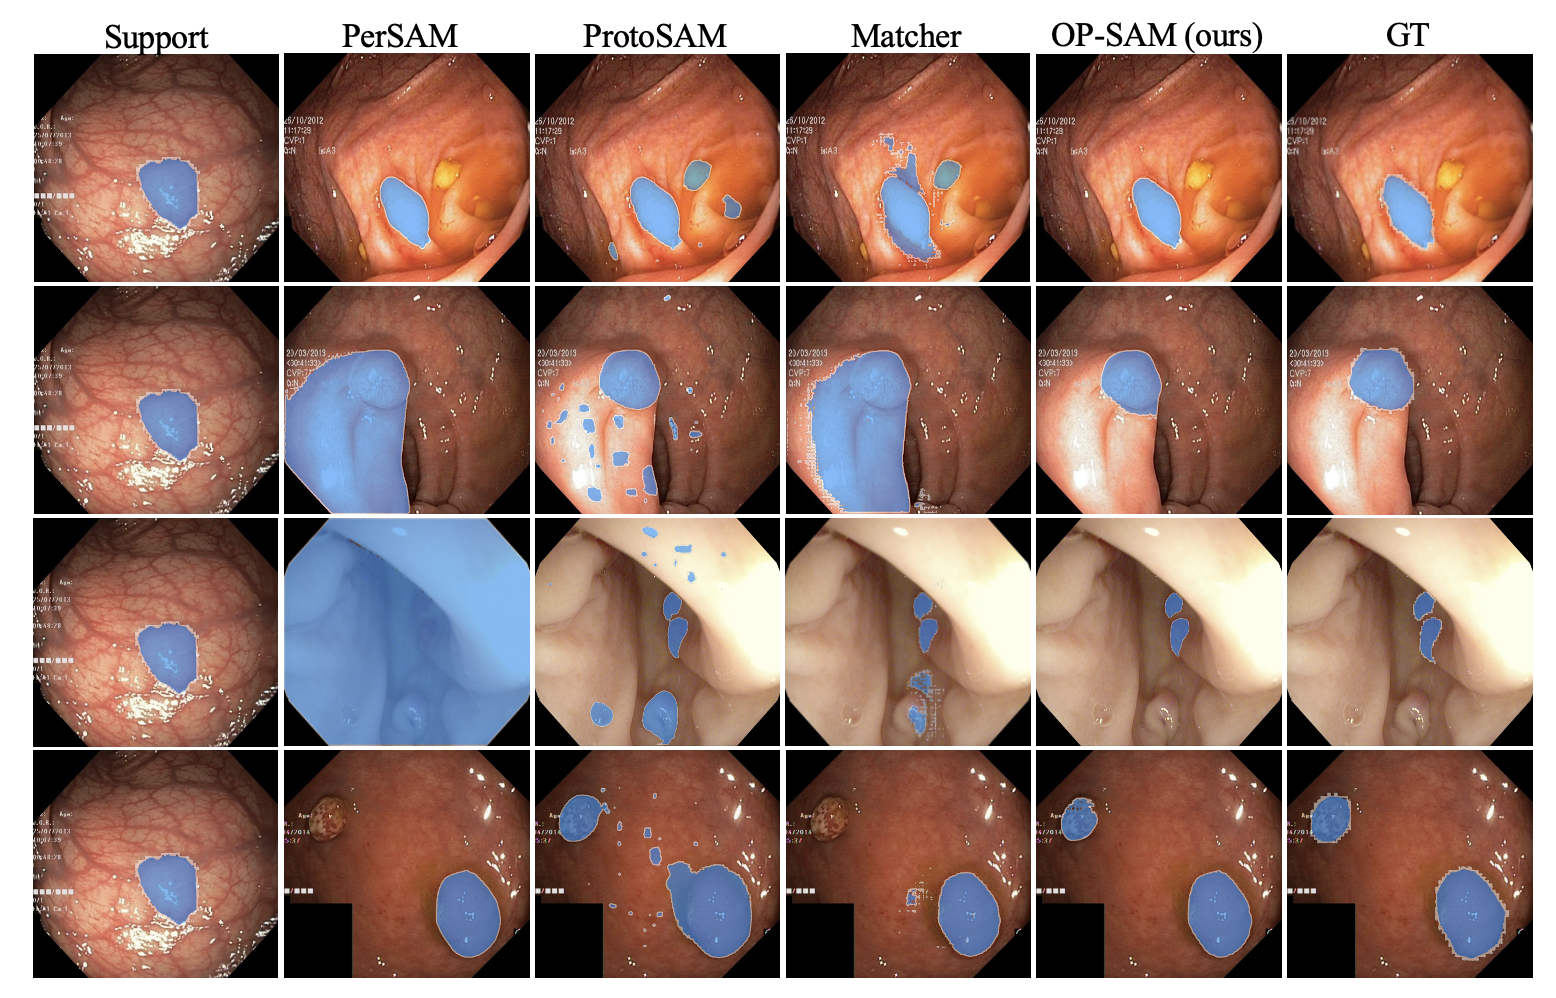}}
    \caption{Qualitative comparison of OP-SAM against state-of-the-art methods. OP-SAM demonstrates enhanced discriminative capability, effectively reducing both false negative and false positive.}
   \label{fig:comp_1}
\end{figure*}

\begin{figure*}[h]
  \centering
   \includegraphics[width=0.9\textwidth]{{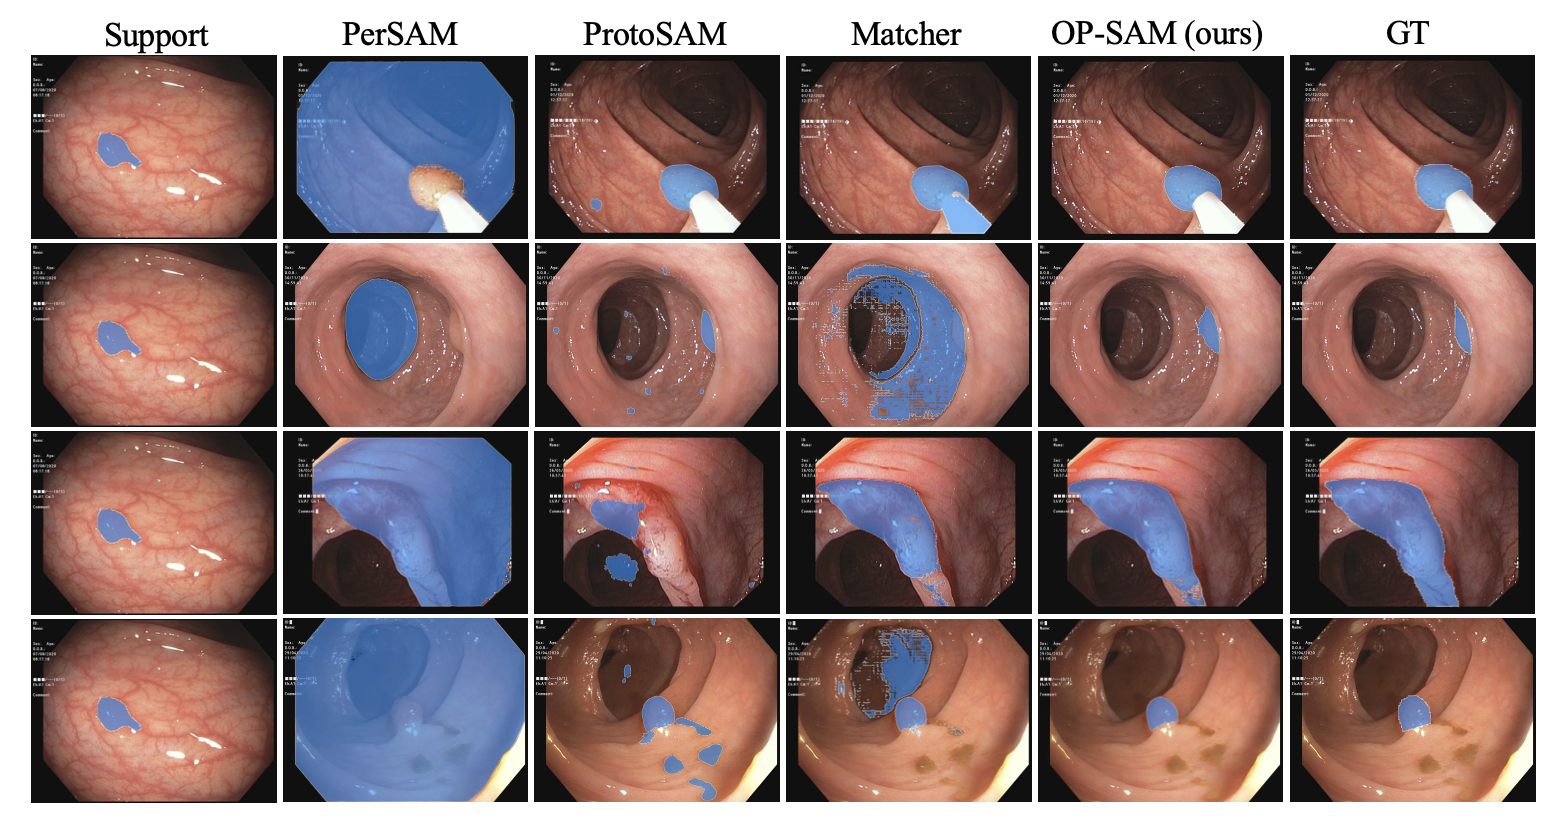}}
    \caption{Qualitative comparison of OP-SAM against state-of-the-art methods. OP-SAM demonstrates superior robustness, maintaining accurate segmentation performance for polyps across various sizes.}
   \label{fig:comp_2}
\end{figure*}
% {
%     \small
%     % \bibliographystyle{ieeenat_fullname}
%     \bibliography{supp}
% }
% % 
% Having the supplementary compiled together with the main paper means that:
% % 
% \begin{itemize}
% \item The supplementary can back-reference sections of the main paper, for example, we can refer to \cref{sec:intro};
% \item The main paper can forward reference sub-sections within the supplementary explicitly (e.g. referring to a particular experiment); 
% \item When submitted to arXiv, the supplementary will already included at the end of the paper.
% \end{itemize}
% % 
% To split the supplementary pages from the main paper, you can use \href{https://support.apple.com/en-ca/guide/preview/prvw11793/mac#:~:text=Delete%20a%20page%20from%20a,or%20choose%20Edit%20%3E%20Delete).}{Preview (on macOS)}, \href{https://www.adobe.com/acrobat/how-to/delete-pages-from-pdf.html#:~:text=Choose%20%E2%80%9CTools%E2%80%9D%20%3E%20%E2%80%9COrganize,or%20pages%20from%20the%20file.}{Adobe Acrobat} (on all OSs), as well as \href{https://superuser.com/questions/517986/is-it-possible-to-delete-some-pages-of-a-pdf-document}{command line tools}.
